# Supplementary material for: Polar Interpolants for Thin-Shell Microstructure Homogenization
Source: arXiv:2505.01779 source file (2025-05-03)
Supplement: Supplementary file 1 [file appendix1.tex]

\section{Appendix}
\label{sec:appendix}

% \subsection{Energy profiles angle-wise}
% \label{sec:appendix:energyprofiles}

% \begin{figure}[h]
%     \centering
%     \includegraphics[width=\linewidth]{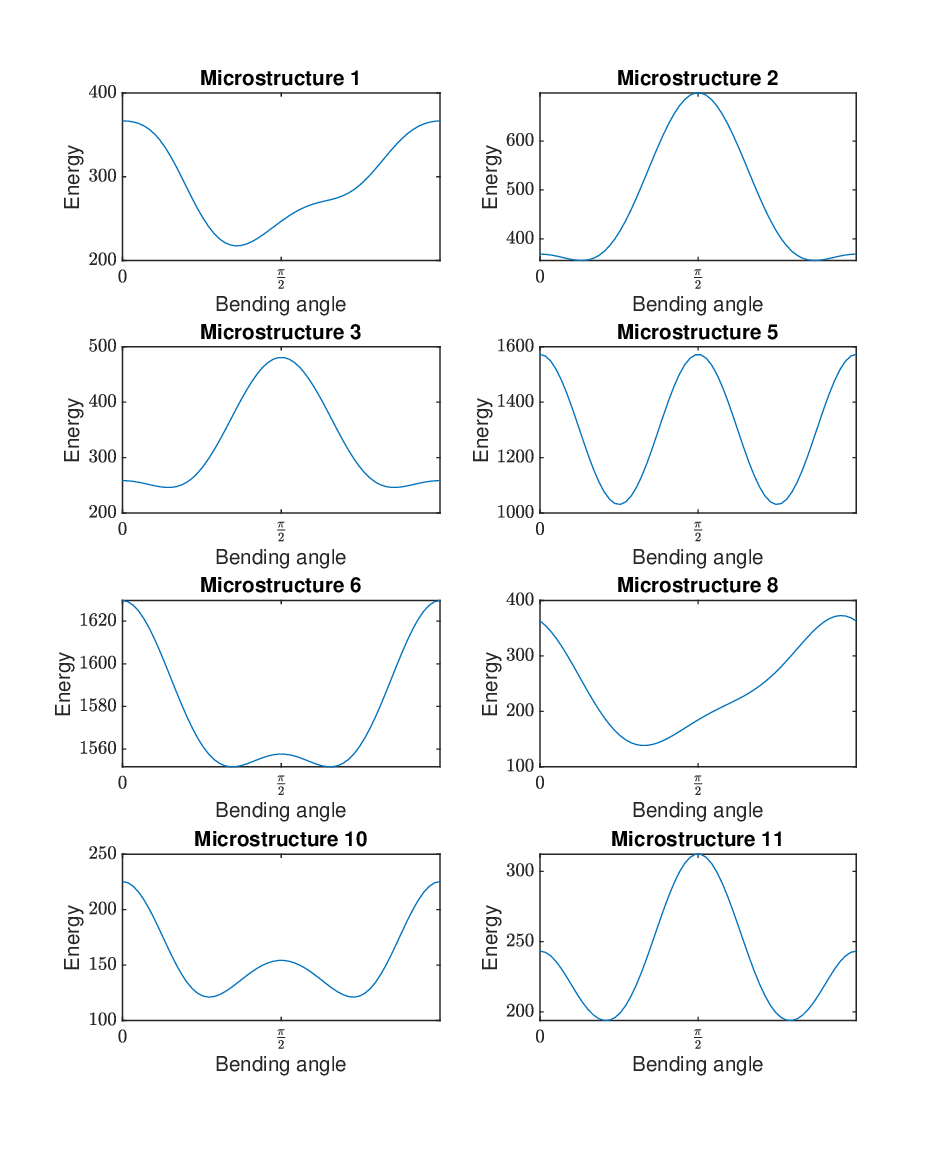}
%     \caption{\Antoine{Microstructures 4 7 9 are not converging. worst case we drop them ?}}
%     \label{fig:my_label}
% \end{figure}

Given a $2 \times 2$ matrix
\[
M = \begin{pmatrix}
A & B \\
C & D \\
\end{pmatrix},
\]
define $\epsilon$ as a small positive number to ensure numerical stability.

Calculate the terms:
\[
S = \sqrt{\left(\frac{A - D}{2}\right)^2 + BC + \epsilon}
\]
\[
\text{cond} = A - D
\]

The eigenvalues are determined by:
\[
\lambda_1 = \frac{A + D}{2} + S
\]
\[
\lambda_2 = \frac{A + D}{2} - S
\]

The angle $\theta$ for the eigenvector is calculated using:
\[
\cos(\theta) = 
\begin{cases} 
\frac{A-D}{2} + S & \text{if } \text{cond} \geq 0 \\
C & \text{otherwise}
\end{cases}
\]
\[
\sin(\theta) = 
\begin{cases} 
B & \text{if } \text{cond} \geq 0 \\
-\frac{A-D}{2} + S & \text{otherwise}
\end{cases}
\]
\[
k = 
\begin{cases} 
-1 & \text{if } \sin(\theta) < 0 \\
1 & \text{otherwise}
\end{cases}
\]
\[
\theta = \arctan2(\sin(\theta) \cdot k, \cos(\theta) \cdot k)
\]

The adjustment with $k$ ensures that the computed angle $\theta$ is correctly confined within the range $[0, \pi]$.

\section{Pruning}
\begin{table}[h!]
\centering
\begin{tabular}{|c|c|c|c|c|c|}
\hline
\textbf{MS} & \textbf{Shape 1} & \textbf{Max} & \textbf{Min} & \textbf{Mean} & \textbf{Std} \\ \hline
mat1 & 130  & 130 & 118 & 129.15 & 1.89 \\ \hline
mat2 & 180  & 180 & 148 & 175.84 & 7.00 \\ \hline
mat3 & 130  & 130 & 119 & 129.28 & 1.97 \\ \hline
mat4 & 500  & 500 & 175 & 381.13 & 76.96 \\ \hline
mat5 & 130  & 130 & 116 & 128.62 & 2.66 \\ \hline
mat6 & 480  & 480 & 188 & 360.81 & 73.39 \\ \hline
mat7 & 280  & 280 & 172 & 246.21 & 31.19 \\ \hline
mat8 & 450 & 450 & 168 & 352.35 & 66.16 \\ \hline
mat9 & 480  & 480 & 178 & 387.51 & 68.78 \\ \hline
mat10 & 450  & 450 & 182 & 366.88 & 62.08 \\ \hline
\end{tabular}
\caption{Statistical Summary of Matrices}
\label{table:stats}
\end{table}

\Antoine{Let's resume the the pruning technique to make sure I understood correctly
\begin{itemize}
    \item  For a given point $x$, I find which interpolants are contributing
    \item in other words, I count how many $ \Psi >1e-7 $ for $w=1$
    \item I repeat this operation, for $x$ = each control point
    \item which gives me a vector of \#activations per entry
    \item from this vector, I output the max,min,mean,std
    \item Almost all interpolants are contributing. It might make sense. $\Psi(k1,k2,d) = \psi(k1,d) +  \psi(k2,d+90)$. We're not only activating the interpolants in the $(k1,k2,d)$ region, but also the ones in $(k1,k2,d+90)$ region.
    \item also, the strain scaling makes the rbf spread in different amplitudes wrt dimension (in other words, we can't consider that a rbf action range is a circle, but an ellipse)
\end{itemize}
}

\Antoine{Even if we have 500 control points in worst cases, we can still defend that it's decent wrt to the high dimension. If we'd sample each dimension uniformly, let's say 5 samples per dimension, we'd have $5^5=3125$ samples}
